# Supplementary material for: Approximate Nearest Neighbors in the Space of Persistence Diagrams
Source: arXiv:1812.11257 source file (2021-03-22)
Supplement: Supplementary file 1 [file appendix.tex]

\appendix
\section{Omitted Proofs}
\label{ap:omitted-proofs}
Here, we provide proofs omitted from the main body of the paper.

\subsection*{Omitted Proofs from~\secref{hashing}}

%%%
\paragraph*{Proof of~\lemref{boundedcollision}}
\begin{proof}
    Recall from \ssref{lattices} that $\delta=\frac{2M}{\eta}$ and
    $|\lattice{M}{2\eta}|=(2\eta)^2 + 2\eta$.

    For the first part, let $P_* \in
    \snap{P}{\nLattice}$ such that
     $\key{P_*}{\nLattice}=\key{Q}{\nLattice}$. Then, we construct a
    matching $\match$ between~$P$ and $Q$ iteratively by peeling off pairs
$(p,q) \in P \times Q$ that are
    mapped to the same grid point $\ell$.
    By \lemref{enumerating}, we
    know that $p$ was snap-rounded to one of the four grid points
    within distance $\delta$ of $p$.
    Additionally, we know that $q$ was snap-rounded to the closest
    grid point.
    Hence, we have $d_{\infty}(p,\ell) \le \delta$
    and $d_{\infty}(q,\ell) \le \frac{1}{2} \delta$.  Thus, by the triangle
inequality,
    we have $d_{\infty}(p,q) \le \delta + \frac{1}{2} \delta = \frac{3}{2}
\delta$;
    an example of this situation is shown in~\subfigref{onecorner}{onecorner-best}.
    Therefore, if $\key{P_*}{\nLattice}=\key{Q}{\nLattice}$, we have $d_B(P,Q)
    \le \frac{3}{2} \delta$.
    %%%

    \begin{figure*}[t!]
        \centering
        \begin{subfigure}[t]{0.45\textwidth}
            \centering
            \includegraphics[]{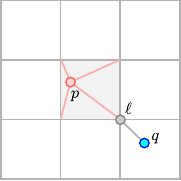}
            \caption{Scenario where in $d_{\infty}(p,q)$ a $P_*$ exists that snaps
            $p$ and $q$ to $\ell$. Notice that $d_{\infty}(p,\ell)
            \le \delta$ and $d_{\infty}(q, \ell)\le \frac{1}{2}\delta$.}
            \label{subfig:onecorner-best}
        \end{subfigure}%
        \hspace{5mm}
        \begin{subfigure}[t]{0.45\textwidth}
            \centering
            \includegraphics[]{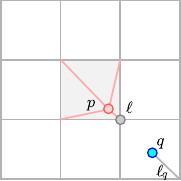}
            \caption{Scenario where $d_{\infty}(p,q)$ is just over $\frac{1}{2}\delta$ but
            $p$ and $q$ do not snap to the same grid point.
            Specifically, $d_{\infty}(p,\ell)
            \le \delta$ and $d_{\infty}(q, \ell) > \frac{1}{2}\delta$.}
            \label{subfig:onecorner-worst}
        \end{subfigure}
        \caption[Boundary-case scenarios for snap-roundings]
        {Illustration for the proof of \lemref{boundedcollision} demonstrating
        the two boundary-case scenarios, where two points are near one another with
        no snap-rounding, and where two points are far from one another but snap-round
        to the same grid point.}
        \label{fig:onecorner}
    \end{figure*}

    To prove the second part, we assume that
    $d_B(P,Q) \le \frac{1}{2} \delta$.
    Recall that $P$ and $Q$ have the
    same number of points and let $\match \subset P \times Q$
    be a perfect matching that
    realizes the bottleneck distance.
    For each pair $(p,q) \in \match$, let $\ell_{q}$ be the grid point to
    which~$q$ snaps in $\key{q}{\nLattice}$, as illustrated in
    \subfigref{onecorner}{onecorner-worst}.
    Then, $d_{\infty}(q, \ell_q) < \frac{1}{2}\delta$ because
    it is the nearest point to $q$.
    Since $d_B(P,Q) \le \frac{1}{2} \delta$,
    we know that $d_{\infty}(p,q) \le \frac{1}{2}\delta$ and $d_{\infty}(p, \ell_q)
    \le d_{\infty}(p,q) + d_{\infty}(q,\ell_q)
    < \delta$ by the triangle inequality which implies that $p$ and $\ell_q$ lie
    in the same grid cell.
    Thus,
    a snap-rounding of $P$ exists such that each~$p$ is snapped to $\ell_q$;
    we denote this snap-rounding~$P_*$. Since $|\match |=|P| = |Q|$ and
    each pair in $\match$ share a grid point in $\key{Q}{\nLattice}$
    and $\key{P_*}{\nLattice}$, we conclude
    that $\key{Q}{\nLattice} = \key{P_*}{\nLattice}$.
\end{proof}
%%%

%%%
\paragraph*{Proof of~\thmref{collision}}
\begin{proof}
    Again, recall from \ssref{lattices} that $\delta=\frac{2M}{\eta}$ and
    $|\lattice{M}{2\eta}|=(2\eta)^2 + 2\eta$.

    We start with the first part.  Let $P_{*}\in
    \delsnap{P}{\nLattice}$
    such that $\key{P_*}{\nLattice}=\key{\widetilde{Q}}{\nLattice}$.
    Then,
    each off-diagonal persistence point $p \in P$ is either snap-rounded to one
    of its neighbors within distance~$\delta$ or deleted in
    order to obtain $P_*$.
    Then, we construct a matching~$\match$ between~$P_*$ and~$\widetilde{Q}$ from
    \lemref{boundedcollision}~Part~\ref{lemPart:snapImpliesBound} with
    bottleneck cost at most~$\frac{3}{2}\delta$; next, we add to the matching
    $\match$ in order to extend the
    matching to a perfect matching between $P$ and $Q$ by considering
    unmatched points of~$Q$
    followed by unmatched points of~$P$.
    Notice that all deleted points of~$Q$ are within~$\frac{1}{2}\delta$
of the diagonal by construction.  Furthermore, all points
in~$P\backslash P_*$ must have
been deleted
    by $\keyfcn$, and hence are within~$\delta$ of
    the diagonal. We
    add all of these pairs (i.e., between $P \backslash P_*$ and the
    diagonal,
and
    between $Q \backslash \widetilde{Q}$ and the diagonal) to~$\match$, thus
    obtaining a perfect matching between~$P$ and $Q$ with bottleneck cost at
    most~$\frac{3}{2} \delta$.

    We now prove the second part.  Assume that $d_B(P,Q)
\leq
    \frac{1}{2}\delta$.
    Let $\match \subset P \times Q$ be a matching that realizes the
    bottleneck distance between $P$ and $Q$.  We use this matching to construct
    a diagram $P_*\in \delsnap{P}{\nLattice}$ by choosing
    which points of $P$ to snap-round to grid points and which points to delete; see
\figref{noisydgm} for an example of the points that
    are eligible for removal during the snap-rounding.
    For each $(p,q) \in \match$ with $q \in \widetilde{Q}$, we
    know that $p \notin \diag$ (recall that $\diag$ denotes the diagonal)
    since $d_B(P,Q) \leq
    \frac{1}{2}\delta$.
    Letting $\ell_q$ be the closest grid point to $q$
    (just as we did in \lemref{boundedcollision}),
    we snap-round $p$ to $\ell_q$ in $P_*$.
    Next, we consider all $(p,q) \in \match$ with $q \notin \widetilde{Q}$
    (i.e., $d_{\infty}(q, D) \le \frac{1}{2} \delta$), where $q$
    is snapped to the diagonal.
    We must show that we can also delete $p$ when constructing
    $P_*\in \delsnap{P}{\nLattice}$, we know~that
    \[ d_{\infty}(p, D) \le d_{\infty}(p,q) + d_{\infty}(q, D) \leq d_B(P,Q)+ \frac{1}{2}
    \delta \leq  \delta,\]
    and so we choose to delete $p$ since it is within $\delta$ of $\diag$
    ($q$ is deleted by the definition of $\widetilde{Q}$).
    Then, we have matched all points in $\widetilde{Q}$ with points in $P$
    and all points that were deleted from $Q$ when obtaining $\widetilde{Q}$
    had their corresponding points in $P$ deleted when constructing $P_*$.
    Therefore, we have constructed a diagram $P_* \in
    \delsnap{P}{\nLattice}$ \mbox{such that
    $\key{\widetilde{Q}}{\nLattice} =  \key{P_{*}}{\nLattice}$}.
\end{proof}
%%%

\subsection*{Omitted proofs from~\secref{approx}}

%%%
\paragraph*{Proof of~\lemref{weakCollision}}
\begin{proof}
It suffices to prove that if $P$ and $Q$ collide in~$\Delta_j$
    then $P$ and~$Q$ collide in $\Delta_{j-1}$.
    From \thmpartref{collision}{snapImpliesBound},
    since $P_j \in \delsnapI{j}{P}$
    and~$\keyI{j}{P_j}=\keyI{j}{\Q_j}$,  a matching~$\match$ exists
    between $P$ and $Q$ such that $\forall (p,q) \in \match$,
    $d_{\infty}(p,q) \leq
    \frac{3}{2} \delta_j$.  We use this matching to find
    $P_{j-1} \in \delsnapI{j-1}{P}$ such that
    $\keyI{j-1}{P_{j-1}}=\keyI{j-1}{\Q_{j-1}}$, which happens when
    there exists a matching $\match' \subset P \times Q$ such that
    for each $(p',q') \in \match'$, either $d_{\infty}(p', \ell_{q}') < \delta_{j-1}$, where
    $\ell_{q}'$ is the closest grid point to $q'$, or
    $\max \{ d(p',D) , 2 d(q',D) \} \leq \delta_{j-1}$.
    Then, we show that we can construct $\match'$.
    We begin with $\match'=\emptyset$, and
    for each $(p,q) \in \match$ we construct one, or more,
    edges and add them to $\match'$.
    To construct each edge, we consider three cases:
    \textsc{Case~$1$}, where $q \in D$;
    \textsc{Case~$2$}, where $p \in D$; and
    \textsc{Case~$3$}, where neither $p$ nor $q$ are in~$D$, which has two subcases.

    \emph{\textsc{Case} $1$ ($q \in D$):}
    Since $(p,q) \in \match$ and $q \in D$, then $p$ is within
    $\delta_j$ of $D$.
    Since $\delta_j = \frac{1}{2}\delta_{j-1}$, we know that $p$
    lies at most $\frac{1}{2}\delta_{j-1}$ from $D$ and can be matched with
    $D$ in a matching corresponding to a collision at $\Delta_{j-1}$ as well.
    Thus, we add $(p,q)$ to $\match'$.

    \emph{\textsc{Case} $2$ ($p \in D$)}:
    Since $(p,q) \in \match$ and $p \in D$, then $q$ is within
    $\frac{1}{2}\delta_j$ of $D$.
    Then, $q$ is at most $\frac{1}{4}\delta_{j-1}$ from $D$, and it can be matched with
    $p\in D$ in a matching corresponding to a collision at~$\Delta_{j-1}$ as well.
    Thus, we add $(p,q)$ to $\match'$.

    \emph{\textsc{Case} $3$ (neither $p$ nor $q$ are in~$D$ in $\Delta_j$):}
    By construction, in level $\Delta_j$, points~$p$ and~$q$ snap to the same grid
    point~$\ell_q$ such that $d_{\infty}(q, \ell_q) \le \frac{1}{2}\delta_j$
    and $d_{\infty}(p, \ell_q) \le
    \delta_j$, since~$q$ is snapped to the
    nearest grid point and~$p$ is snapped to one of the four nearest
    grid~points.

    \emph{\textsc{Subcase} $3a$ ($d_{\infty}(q,D)\le \frac{1}{2}\delta_{j-1}$)}.
    We add $(\proj(q),q)$ to $\match'$, since $q$ must be snap-rounded to $D$ in
    $\Delta_{j-1}$.
    In order to match $p$ in $\match'$,
    we show that $p$ also has a snap-rounding to $D$
    in level~$\Delta_{j-1}$.
    Since $d_{\infty}(q,D)\le \frac{1}{2}\delta_{j-1}$, we know that either
    $d(\ell_q,D)=\delta_j = \frac{1}{2}\delta_{j-1}$ or
    $d(\ell_q,D)=\frac{1}{2}\delta_j = \frac{1}{4}\delta_{j-1}$.
    Since $d_{\infty}(p, \ell_q) \le \delta_j = \frac{1}{2}\delta_{j-1}$,
    the triangle inequality implies that $d(p,D) \leq \delta_{j-1}$.
    Therefore,~$p$ can be deleted in the snap-rounding in $\Delta_{j-1}$,
    so we add $(p,\proj(p))$ to $\match'$.

    \emph{\textsc{Subcase} $3b$ ($d_{\infty}(q,D)>\frac{1}{2}\delta_{j-1}$)}.
    Let $\ell'_{q}$ be the grid point in level $\Delta _{j-1}$ to which $q$ snap-rounds.
    Since $q$ is more than $\frac{1}{2}\delta_{j-1}$ from $D$,
    $d_{\infty}(\ell_q, \ell'_{q}) \le \frac{1}{2}\delta_{j-1}$, which implies
    that $d_{\infty}(p, \ell'_{q})
    \le  \delta_j + \frac{1}{2}\delta_{j-1}
    \leq \delta_{j-1}$ by the triangle inequality.
    Therefore, we can snap-round $p$ to~$\ell'_{q}$ in $\Delta_{j-1}$.
    So, we add $(p,q)$ to $\match'$.

    Finally, we find $P_{j-1} \in \delsnapI{j-1}{P}$ as follows:
    for every $(p,q) \in \match'$ such that $p$ is off-diagonal,
    we either (1) delete $p$ if $q$ is on
    $D$, or (2) snap-round $p$ to the grid
    point in~$\Delta_{j-1}$ nearest to $q$.  Therefore, we conclude that if
    $P$ and $Q$ collide at $\Delta_j$, then $P$ and $Q$ also collide at
    $\Delta_{j-1}$.
\end{proof}
%%%

%%%
\paragraph*{Proof of~\lemref{nnBin}}
\begin{proof}
Assume that $P^{nn}$ does not have a collision with $\keyI{i-2}{\Q_{i-2}}$.
By the contrapositive of \thmpartref{collision}{boundImpliesSnap},
$2\delta_i = \frac{1}{2}\delta_{i-2} < d_B(P^{nn},Q)$.
As $Q$ collides with $P$ in $\Delta_i$,
by \thmpartref{collision}{snapImpliesBound},
$d_B(P,Q)\le \frac{3}{2}\delta_i$.
Combining the inequalities, we get
$d_B(P,Q)\le \frac{3}{2}\delta_i < 2\delta_i < d_B(P^{nn},Q)$,
which implies that $P^{nn}$ is not the nearest neighbor, a contradiction.
\end{proof}
%%%

%%%
\paragraph*{Proof of~\lemref{nn}}
\begin{proof}
Let $P\in \Gamma$ and $P_i \in \delsnapI{i}{P}$ such that
$\keyI{i}{P_i}=\keyI{i}{\Q_i}$. In other words, $P_i$ is a snap-rounding of
 $P$ that collides with $Q$ at level~$i$.
By \lemref{nnBin}, $P^{nn}$ has a snap-rounding in
$\Delta_{i-2}$ colliding with $Q$.
And, by our assumption, as $Q$ has no collisions in level $i+1$,
$P^{nn}$ may have its last collision with $Q$ in
$\Delta_{i-2}$, $\Delta_{i-1}$, or $\Delta_{i}$.
To bound the bottleneck distance,
we must only consider the worst-case scenario, where
$d_B(P^{nn}, Q)$ is as small as possible and $d_B(P,Q)$ is as large as possible.
As $P$ and $Q$ collide in level $i$,
by \thmpartref{collision}{snapImpliesBound},
$d_B(P,Q) \le \frac{3}{2} \delta_i$.
And, by the contrapositive of \thmpartref{collision}{boundImpliesSnap},
    if the last collision of $P^{nn}$ and $Q$ is:
in $\Delta_{i-2}$, then
    $\delta_i = \frac{1}{2}\delta_{i-1} < d_B(P^{nn}, Q)$;
in $\Delta_{i-1}$, then
   $\frac{1}{2}\delta_{i} < d_B(P^{nn}, Q)$; or
in $\Delta_{i}$, then
    $\frac{1}{4}\delta_i = \frac{1}{2}\delta_{i+1} < d_B(P^{nn}, Q)$.
Therefore,
\[
    \frac{1}{2}\delta_{i+1}
    < d_B(P^{nn},Q)
    \le d_B(P,Q)
    \le \frac{3}{2}\delta_i
    = 6\left( \frac{1}{2} \delta_{i+1} \right)
    < 6 \big(d_B(P^{nn}, Q)\big),
\]
which implies that
every diagram $P$ with a key in $\Delta_i$ colliding with $\keyI{i}{\Q}$
is a six-approximation of the nearest neighbor of~$Q$ in terms of
bottleneck distance.
\end{proof}
%%%

%%%
\paragraph*{Proof of~\lemref{knnLoc}}
\begin{proof}
Assume, for contradiction, that $P^k$ does not have a collision with $Q$ in $\Delta_{i-2}$.
By the contrapositive of \thmpartref{collision}{boundImpliesSnap},
$2\delta_i = \frac{1}{2}\delta_{i-2} < d_B(P^k,Q)$.
Furthermore,
by \thmpartref{collision}{snapImpliesBound},
if a diagram $P\in \Gamma$ collides with $Q$ in $\Delta_i$,
then $d_B(P,Q)\le \frac{3}{2}\delta_i$.
Since there are at least $k$ collisions with $Q$ in $\Delta_i$, there
must be $k$ diagrams with bottleneck distance less than
or equal to $\frac{3}{2}\delta_i < 2\delta_i < d_B(P^k,Q)$.
The previous statement, however, is a contradiction to the
claim that $P^k$ is the $k$th nearest neighbor of $Q$ with respect to
bottleneck distance.
\end{proof}
%%%

%%%
\paragraph*{Proof of~\lemref{kNNDepth}}
\begin{proof}
If $P^k$ has a snap-rounding that collides with $Q$ in any $\Delta_j$ for $j > i+2$
then it will also have a snap-rounding colliding with $Q$ in $\Delta_{i+3}$ by
\lemref{weakCollision}.
Therefore, it suffices to show that $P^k$ does not collide with $Q$ in $\Delta_{i+3}$.
Then, suppose, by contradiction, that $P^k$ has a snap-rounding that collides with $Q$
    in $\Delta_{i+3}$.  Then, by \thmpartref{collision}{snapImpliesBound}, we know that $d_B(P^k,Q) \leq
    \frac{3}{2} \delta_{i+3}= \frac{3}{8} \delta_{i+1} < \frac{1}{2}
    \delta_{i+1},$ which implies that at least $k$ diagrams in $\Gamma$ have
    distance at most $\frac{1}{2}\delta_{i+1}$ from $Q$.   Furthermore, by
    \thmpartref{collision}{boundImpliesSnap}, we
    know that all $P \in \Gamma$ such
    that $d_B(P,Q) \leq \frac{1}{2} \delta_{i+1}$ collide with $Q$ in~$\Delta_{i+1}$.
    Hence, $Q$ has at least $k$ collisions in
    $\Delta_{i+1}$, which contradicts our choice of $i$.
\end{proof}
%%%

%%%
\paragraph*{Proof of~\thmref{approxnn}}
\begin{proof}
We begin by describing how we can use the previous lemmas to organize and
    search~$\bigds$.  \lemref{weakCollision} tells us that for $i < j$,
$\keyI{j}{\Q _i} \in \Delta_j$ then $\keyI{i}{\Q _i} \in \Delta_i$
which implies that~$\bigds$ can be ordered by $i \in \{ 0, \ldots,
\tau \}$.
Using the ordering, we can perform a binary search to find the largest $i$
such that~$\keyI{i}{\Q _i} \in \Delta_i$.
Every diagram with a key in~$\Delta_i$ colliding with $\keyI{i}{\Q _i}$
is a six-approximation of the nearest neighbor of~$Q$ by
\lemref{nn}.

We begin by analyzing the space of $\bigds$.
The structure contains $\tau$ levels. For each level, we store, in
increasing order, the $O(5^m)$ snap-roundings for each of the $n$
persistence diagrams.  So, the total space \mbox{of $\bigds$ is $\spcone$.}

Next, we consider the complexity of finding a six-approximation of
the nearest neighbor for $Q$.
Searching for the largest $i$ such that $\keyI{i}{\Q _i} \in \Delta_i$
requires a binary search through $\bigds$ and another binary
search through each~$\Delta_i$ that is encountered to search for a collision.

The time for each search in~$\Delta_i$ is analyzed using three observations.
First, generating a key for~$Q$, i.e., $\keyI{i}{\Q _i}$ takes $O(m)$ time.
Second, comparing the keys of two diagrams takes $O(m)$ time.
Third, let $n=|\Gamma|$, since each diagram has $O(5^m)$ hashes, each $\Delta_i$ has at
most $O(n5^m)$ keys.
Using these three observations,
we get that searching $\Delta_i$ takes $O(m + m\log(n5^m))$.
The search time can be simplified. Since,
$m\log(n5^m) = m\log(n) + m^2\log(5)$,
the search at each~$\Delta_i$ is
$O(m + m\log(n) + m^2) = O(m\log(n) + m^2)$ time.
Since we search~$O(\log(\tau))$ levels of $\bigds$,
and the search at each level is $O(m\log(n) + m^2)$, the
total query time is $\qtone$.
\end{proof}
%%%

%%%
\paragraph*{Proof of~\lemref{knnApprox}}
\begin{proof}
Let $P \in \Gamma$ and $P_i \in \delsnapI{i}{P}$ such that
    $\keyI{i}{P_i}=\keyI{i}{\Q_i}$.
That is, $P$ is one of the~$k$ distinct diagrams
    that collide with $Q$ at level $i$.
By \corref{kNNLevels},
    $P^k$ has a collision with $Q$ in
    $\Delta_{i-2}$, $\Delta_{i-1}$,
    $\Delta_{i}$, $\Delta_{i+1}$,
    or $\Delta_{i+2}$.
To bound the bottleneck distance,
    we must only consider the worst-case scenario,
    in which $d_B(P^k, Q)$ is as small as possible
    and $d_B(P,Q)$ is as large as possible.
As $P$ and $Q$ collide in level $i$,
    by \thmpartref{collision}{snapImpliesBound},
    $d_B(P,Q) \le \frac{3}{2} \delta_i$.
And, by the contrapositive of \thmpartref{collision}{boundImpliesSnap},
    for $\alpha \in \{ -2, -1, \ldots, 2\}$,
    if the last collision of $P^{k}$ and $Q$ is in $\Delta_{i+\alpha}$,
    then ${2^{-2-\alpha}}\delta_i < d_B(P^k, Q)$.
The distance is smallest when $\alpha = 2$, that is,
    $\frac{1}{16}\delta_i < d_B(P^k, Q)$.
Therefore,
\[
    d_B(P,Q)
    \le \frac{3}{2}\delta_i
    = 24 \left( \frac{1}{16} \delta_{i} \right)
    < 24 \big( d_B(P^k,Q) \big),
\]
which implies that
every diagram $P$ with a key in $\Delta_i$ colliding with $\keyI{i}{\Q}$
is a $24$-approximation of the $k$th nearest neighbor of~$Q$ in terms of
bottleneck distance.
\end{proof}
%%%

%%%
\paragraph*{Proof of~\corref{approxkNN}}
\begin{proof}
We begin by searching to find the largest $i$ such that:
    $\keyI{i}{\Q_i}\in \Delta _i$,
    and the list of diagrams at key $\keyI{i}{\Q_i}$ is of at least length $k$.
We can still utilize binary search to traverse the levels of $\bigds$.
At each level, however, once a matching key is found, we must determine if there are $k$ unique neighboring keys with the same value.
Recall that at each key, we stored the count of the number of unique diagrams.
Thus, we can determine the number of unique diagrams hashed to a particular key in
constant time.
Then, searching each level $\Delta_i$ takes time $O(m\log(n) + m^2)$ from~\thmref{approxnn}.
Once the largest $i$ with $k$ colliding diagrams is found, we return any $k$
diagrams from the list at $\keyI{i}{\Q_i}$.
Any of these colliding diagrams will be a $24$-approximation of the $k$th nearest
neighbor of $Q$ by~\lemref{knnApprox}.
Finding $k$ diagrams from the list at $\keyI{i}{\Q_i}$ takes time $O(k)$ time,
so the total time
complexity for searching and returning $k$ diagrams at a particular level
is $O(m\log(n) + m^2 + k)$, making
the overall time complexity for searching $\qtknn$.
No modifications need to be
made to~$\bigds$ to support these queries so the space complexity remains
the same from~\thmref{approxnn}.
\end{proof}
%%%
